# Supplementary material for: Resonantly Interacting Fermi-Fermi Mixture of $^{161}$Dy and $^{40}$K
Source: arXiv:1909.03424 ancillary file (2020-04-02)
Supplement: Supplementary file 1 [file SuppMat-DyK-reso.pdf]

# Supplemental Material:
# Resonantly Interacting Fermi-Fermi Mixture of $^{161}$Dy and $^{40}$K

C. Ravensbergen,[1,2] E. Soave,[1] V. Corre,[1,2] M. Kreyer,[1] Bo Huang (黄博),[1,2] E. Kirilov,[1] and R. Grimm[1,2]

[1] *Institut für Experimentalphysik, Universität Innsbruck, 6020 Innsbruck, Austria*
[2] *Institut für Quantenoptik und Quanteninformation (IQOQI), Österreichische Akademie der Wissenschaften, 6020 Innsbruck, Austria*

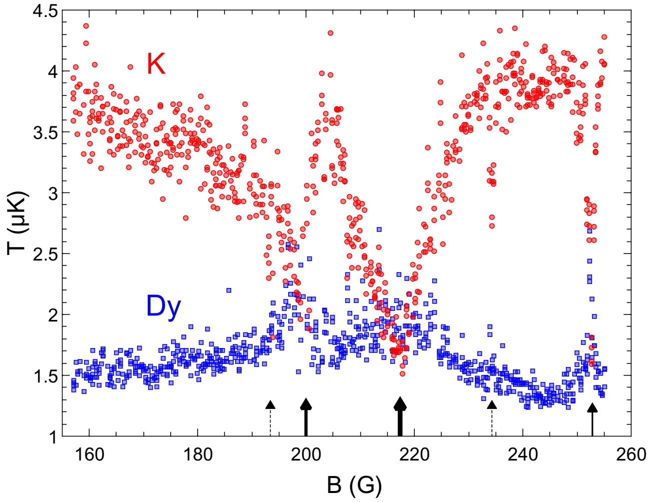


FIG. 1. Thermalization scan revealing magnetic-field dependent resonances in interspecies elastic scattering. The mixture is initially prepared in a non-equilibrium situation, where the $^{161}$Dy component (1.3 $\mu$K) is much colder than the $^{40}$K component (4 $\mu$K). Within a short hold time of 50 ms, interspecies thermalization is observed. Fast thermalization is found to reach essentially equal temperatures at three points (solid arrows), which reveals the existence of three relatively broad Feshbach resonances. Indications of further, much narrower resonances are observed as well (two examples marked by dashed arrows). The broadest resonance, centered near 217 G is the one of main interest for the creation of strongly interacting Fermi-Fermi systems.

## I. FESHBACH RESONANCE SCENARIO

To date, no theoretical model is available that would describe the scattering properties of our Dy-K mixture. Our experimental characterization in the region of interest therefore relies on a combination of various observables, like the positions of resonance poles and zero crossings, and measurements of the interspecies thermalization time. Our basic model assumption is a scenario of three partially overlapping $s$-wave Feshbach resonances.

### A. Wide-range thermalization scan

Figure 1 shows a thermalization scan over the wide magnetic field range from 155 to 255 G. After evaporatively cooling the mixture at low magnetic fields down to a temperature of about 1.3 $\mu$K, a short period (60 ms) of species-selective parametric heating by trap power modulation was applied to increase the temperature of the $1.4{\times}10^4$ K atoms to about 4 $\mu$K, leaving the temperature of the $2.9{\times}10^4$ Dy atoms essentially unchanged. For carrying out the measurements in the high-field region, we then quickly (within 12 ms) ramped up the magnetic field to the variable target field, where (partial) thermalization took place. After a hold time of 50 ms, the magnetic field was quickly (within 1 ms) ramped to 235.4 G. At this field, chosen for thermometry, the interspecies interaction is very weak and the sample expands ballistically after release from the trap. Temperatures were measured by standard time-of-flight imaging.

The thermalization scan reveals a scenario dominated by three broad Feshbach resonances, at the centers of which very fast interspecies heat exchange occurs and the temperatures become nearly equal. The corresponding positions are located near 200, 217, and 253 G (see solid arrows in Fig. 1). While the first resonance (near 200 G) is quite strong and has considerable overlap with the 217-G resonance (second resonance), the third resonance (near 253 G) is clearly weaker and well separated from the two other ones. Further, much narrower resonances exist (dashed arrows), with negligible effect on the overall scenario.The resonance near 217 G is the strongest one and thus the feature of main interest in our present work.

### B. Model of three overlapping resonances

The magnetic-field dependence of the scattering length in a scenario of overlapping Feshbach resonances, assuming a constant background $a_{\rm bg}$, can be represented by the product formula [1, 2]

$$a(B) = a_{\rm bg} \prod_{i=1}^{n} \frac{B - c_i}{B - p_i}\,, \tag{1}$$

where the parameters $p_i$ and $c_i$ denote the positions of the poles and zero crossings, respectively. A straightforward transformation gives the equivalent sum formula [2]

$$a(B) = a_{\rm bg} \left( 1 - \sum_{i=1}^{n} \frac{\delta_i}{B - p_i} \right) \tag{2}$$

with

$$\delta_i = (c_i - p_i) \prod_{j \neq i}^{n} \frac{c_j - p_i}{p_j - p_i} . \quad (3)$$

A practical advantage of the product formula is that it explicitly contains the positions $c_i$ of the zero crossings, which are often good observables in an experiment [3, 4]. An advantage of the sum formula is that the parameters $\delta_i$ provide a measure for the relative strengths of the different resonance contributions. In the case of a single, isolated resonance $\delta_1 = c_1 - p_1$ corresponds to the common definition [5] of the Feshbach resonance width.

### C. Determination of poles and zero crossings

The poles (zero crossings) associated with Feshbach resonances can be identified as points of fastests (slowest) thermalization in scans like the one shown in Fig. 1. We have carried out further scans with higher resolution in narrower magnetic field ranges near the resonance centers, and obtained values $p_1 = 200.1(2)$ G and $p_2 = 217.27(15)$ G for the poles of the two broadest resonances. Here, because of the fast thermalization, we used short hold times of 50 ms (15 ms) for the determination of $p_1$ ($p_2$).

For the observation of zero crossings, close to which thermalization is very slow, long hold times are favorable. In a scan with a hold time of 1.2 s, we determined the position $c_1 = 203.0(2)$ G for the zero crossing between the poles $p_1$ and $p_2$.

The third resonance (near 253 G) is found in a region where the local background scattering length is very small. This is a consequence of the near cancellation of the the global background scattering length $a_{\rm bg}$ by the effect of the two broad resonances. While the pole position $p_3$ can be determined in a straightforward way from the point of fastest thermalization, a determination of the two zero crossings $c_2$ and $c_3$ solely based on the observation of thermalization minima turns out to be rather inaccurate. We therefore investigated thermalization in a wide range covering $c_2$, $p3$, and $c_3$ and analyzed the resulting data based on the model introduced in Ref. [6] and applied to our mixture in [7] (see also Sec. I E).

The model is based on the assumption of thermalization described by an exponential decrease of the temperature difference with increasing hold time, with a relaxation rate being proportional to the elastic scattering cross section and thus being proportional to $a^2(B)$. The temperature difference $\Delta T = T_{\rm K} - T_{\rm Dy}$ can then be written as a function of the magnetic field strength,

$$\Delta T(B) = \Delta T_0 \exp[-C a^2(B)] , \quad (4)$$

where $\Delta T_0$ is the initial temperature difference. The parameter $C$ is proportional to the hold time and further determined by a combination of the experimental parameters, as described in Refs. [6, 7].

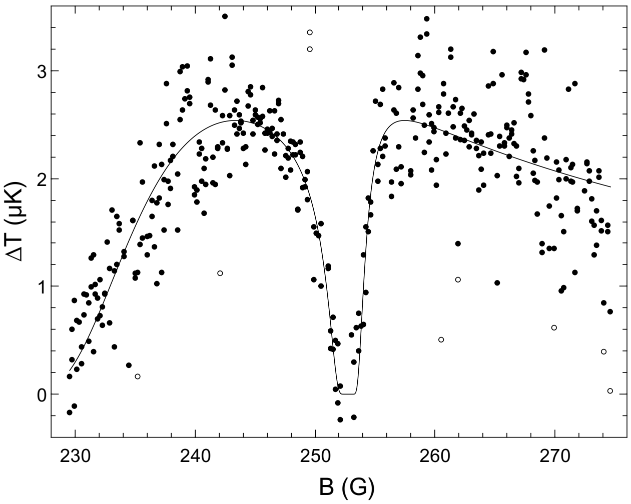


FIG. 2. Thermalization scan in the region of the third resonance. The temperature difference $\Delta T$ was measured for a long hold time of 1.2 s. The solid line represents a fit based on the thermalization model described in the text, from which we obtain the pole position (minimum of $\Delta T$) and the positions of the two neighboring zero crossings (maxima). Note that we have applied a rejection algorithm based on repeated application of Chauvenet's criterion [8] to reduce the effect of outliers and barely resolved narrow Feshbach on the fit. This removed 17 data points (open symbols) of in total 393 data points and resulted in a very robust parameter values.

The measurements in Fig. 2 were taken in a wide range between 229 and 275 G under similar initial conditions as in Fig. 1, but with a much longer hold time of 1.2 s. Thermometry was performed in the same way as in Fig. 1. We fitted the data based on the thermalization model [Eq. (4)] and the product formula [Eq. (1)] for $a(B)$. The parameters $p_1$, $p_2$, and $c_1$ were fixed to their separately determined values (see above discussion). The fit (solid curve in Fig. 2) yielded the parameter values $p_3 = 252.79(8)$ G, $c_2 = 243.4(4)$ G, and $c_3 = 257.5(4)$ G.

The complete set of resonance parameters $p_i$ and $c_i$ for our three-resonance model is summarized in Table I. Based on Eq. (3), we also calculated the parameters $\delta_i$, which characterize the strengths of the resonances. The resulting values (last column) confirm that the second resonance is the strongest one. The first resonance is about three times weaker, and the third resonance is about 20 times weaker than the strongest one.

### D. Background scattering length

Having determined the poles and zero crossings describing our three-resonance scenario, the remaining task is to determine the background scattering length $a_{\rm bg}$, which is left as the only unknown quantity in Eqs. (1) and (2). For this purpose, we carried out thermalization measurements in a similar way as described in Ref. [7].

TABLE I. Parameters characterizing the scenario of three overlapping resonances. The given $1\sigma$ uncertainties include the fit errors and estimates for model-dependent errors. Additional magnetic-field uncertainties from the calibration and from day-to-day fluctuations are estimated on the order of 0.1 G.

| $i$ | $p_i$ (G) | $c_i$ (G) | $\delta_i$ (G) |
|---|---|---|---|
| 1 | 200.1(2) | 203.0(2) | 7.9(7) |
| 2 | 217.27(15) | 243.4(4) | 24.6(6) |
| 3 | 252.79(8) | 257.5(4) | 1.2(1) |

We selected magnetic field regions, where thermalization takes place on experimentally convenient timescales and which are free of narrow Feshbach resonances, and determined the absolute values $|a(B)|$ of the scattering length for nine different values of the magnetic field strength. The corresponding signs uniquely follow from our three-resonance model. In this way, we obtained the nine measured values shown in Fig. 3. We finally fitted Eq. (1) to these data points with $a_{\rm bg}$ being the only free parameter. This yields the value of $a_{\rm bg} = +59(3)\, a_0$, where the given uncertainty includes the fit error and the effect of the uncertainties in the resonance parameters $p_i$ and $c_i$.

We estimate that systematic uncertainties in the experimental parameters (mainly uncertainties in the atom numbers and trap frequencies) and model-dependent errors result in an additional relative uncertainty of 15%, which dominates the error budget. Therefore, our final result for the background scattering length in the 200-G region is $a_{\rm bg} = +59(9)\, a_0$. It is interesting to note that our previous measurement [7], which was carried out at a low magnetic field of 430 mG, gave essentially the same value ($|a_{\rm bg}| \approx 60\, a_0$) , although the background scattering length may slowly vary with the magnetic field.

### E. Analysis of thermalization measurements

The basic idea of our cross-species thermalization measurements to determine the Dy-K elastic scattering cross section (see example in Fig. 4) is the same as reported in [7], but here we have to deal with the additional complication that strong Dy losses occur during the thermalization process.

Our model was originally introduced in [6] and can be expressed in terms of a differential equation for the temperature difference $\Delta T = T_{\rm K} - T_{\rm Dy}$,

$$\frac{d}{dt}\Delta T = -\sigma_{\rm el}^2 \frac{\xi q}{3\pi^2} \frac{m_{\rm Dy}\bar{\omega}_{\rm Dy}^3}{k_{\rm B} T_{\rm Dy}} (N_{\rm Dy} + N_{\rm K})\, \Delta T, \qquad (5)$$

where $\sigma_{\rm el} = 4\pi a^2$ is the cross section for elastic Dy-K collisions and $\xi = 4 m_{\rm Dy} m_{\rm K}/(m_{\rm Dy} + m_{\rm K})^2$ accounts for the effect of mass imbalance in the collisional energy transfer. The factor $q$ depends on the ratio of polarizabilities, masses, and temperatures [7]. Under our experimental conditions, this factor can be well approximated by a constant $q = 1.45$.

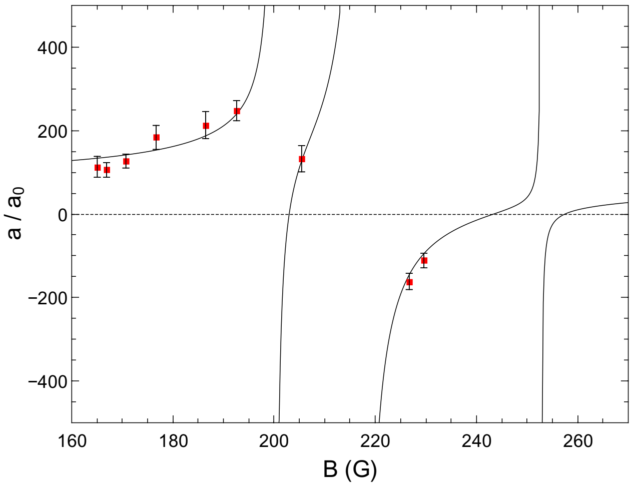

FIG. 3. Magnetic-field dependence of the scattering length in the range of interest. The solid lines represent our model of three overlapping Feshbach resonances, with all parameters being determined experimentally. The experimental data points result from measurements of the scattering cross section by interspecies thermalization.

A typical data set for the time evolution of the atom numbers $N_{\rm Dy}$, $N_{\rm K}$ and the temperatures $T_{\rm Dy}$, $T_{\rm K}$ is shown in Fig. 4(a) and (b). As a first step in the analysis, we independently fit the observed decay of $N_{\rm Dy}$, the slow decrease of $N_{\rm K}$, and the increase in $T_{\rm Dy}$ with simple exponential model functions, which we generally find to describe the data well. As a second step, we fit a numerical solution of Eq. (5) to the decreasing temperature difference $\Delta T$, with the evolution of $T_{\rm Dy}$ and $N_{\rm Dy} + N_{\rm K}$ described by the fit functions obtained before. Figure 4(c) illustrates that the fit with the two free parameters $\sigma_{\rm el}$ and $\Delta T_0$ matches the experimental data very well. For our specific example ($B = 229.5$ G, $\bar{\omega}_{\rm Dy}/2\pi = 180$Hz), we obtain a best estimate for $\sigma_{\rm el}$ corresponding to $|a| = 87\, a_0$.

### F. 217-G resonance: Strength and universal range

For the experiments described in the main text, we are mainly interested in the interspecies scattering length near the pole of the 217-G resonance. Here, the scattering length can be well approximated by

$$a(B) = -\frac{A}{B - B_0}\, a_0\,, \qquad (6)$$

where $B_0 = p_2 = 217.27(15)$ G and $A = \delta_2\, a_{\rm bg}/a_0 = +1450(230)$ G.

For discussing the character of this Feshbach resonance in terms of entrance-channel or closed-channel dominated behavior [5], it is useful to introduce a characteristic

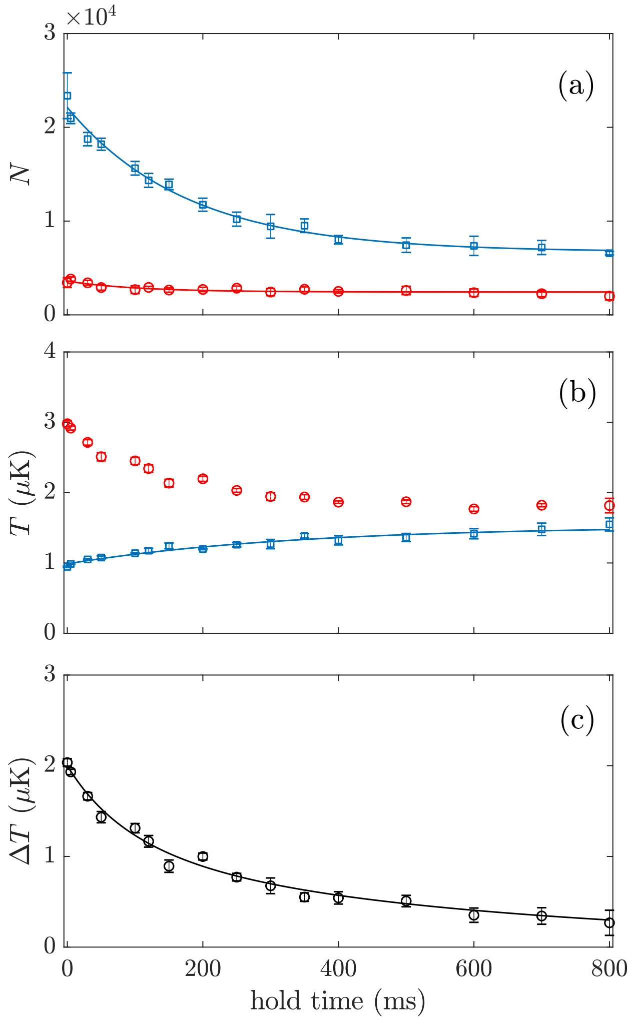


FIG. 4. Example for cross-species thermalization ($B = 229.5\,\mathrm{G}$) and the fit analysis to extract a value for $|a|$. (a) Observed time evolution of the atom numbers $N_{\mathrm{Dy}}$ (blue open squares) and $N_{\mathrm{K}}$ (red open circles) together with fits by simple exponential functions with a constant offset. (b) Time evolution of the temperatures $T_{\mathrm{Dy}}$ and $T_{\mathrm{K}}$; the increasing Dy temperature is again fitted by a simple heuristic model function. (c) Evolution of the temperature difference $\Delta T = T_{\mathrm{K}} - T_{\mathrm{Dy}}$ with a numerical fit based on Eq. (5).

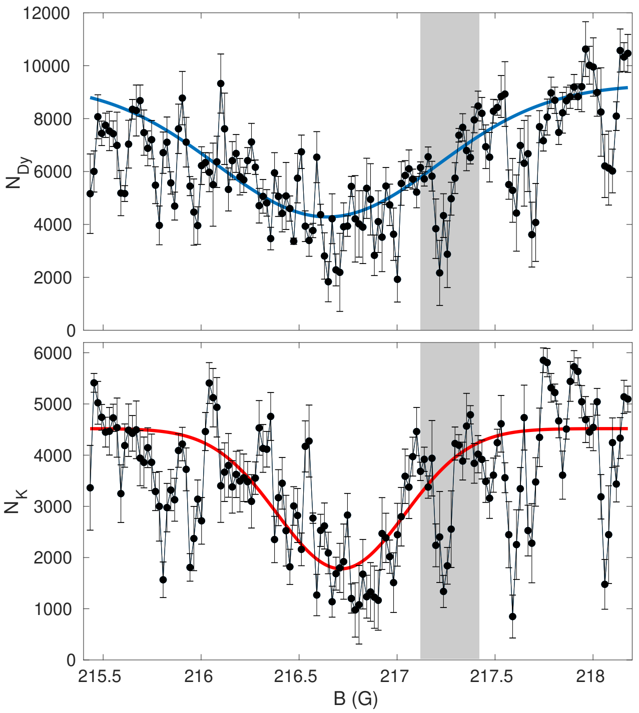


FIG. 5. Loss scan in the resonance region. The plots show the number of Dy atoms (upper panel) and K atoms (lower panel) left in the trap ($\bar{\omega}_{\mathrm{Dy}} = 2\pi \times 130\,\mathrm{Hz}$) after a of hold time 150 ms at a fixed magnetic field. The initial atom numbers are $N_{\mathrm{Dy}} = 24\,000$ and $N_{\mathrm{K}} = 6000$, and the initial temperature is $T = 500\,\mathrm{nK}$. The solid lines are Gaussian fits to the broad loss feature, excluding narrow loss features. The shaded region indicates the $1\sigma$-uncertainty in our knowledge of the pole position of the strong 217-G resonance.

length as defined by the range parameter [9]

$$R^* = \frac{\hbar^2}{2m_{\mathrm{r}} a_0\, \delta\mu\, A}\,. \tag{7}$$

Here $m_{\mathrm{r}} = 32.04\,\mathrm{a.m.u.}$ is the reduced mass and $\delta\mu$ the (unknown) differential magnetic moment. The universal range of a Feshbach resonance is reached if $|a| \gg R^*$, which also represents a necessary condition for a strong Pauli suppression of few-body losses [10].

The properties of the molecular states underlying our Feshbach resonances are currently unknown and require further in-depth investigation. For now, to get an idea of the universal range, we use a conservative guess for the differential magnetic moment $\delta\mu = 0.1\,\mu_{\mathrm{B}}$, where $\mu_{\mathrm{B}}$ is Bohr's magneton. This yields $R^* \approx 300\,a_0$ as a conservative estimate for the range parameter. We thus conclude that the universality condition $|a| \gg R^*$ is rather easy to fulfill near the pole of our 217-G Feshbach resonance. We note that also the many-body condition $k_F R^* \ll 1$ for universality in a fermionic system (Fermi wave number $k_F$) is well fulfilled under realistic conditions.

## II. DECAY

### A. Overview of losses in the resonance region

The loss scan in Fig. 5 presents an overview of the complex magnetic-field dependence of losses in the region of the 217-G resonance. Here the number of Dy and K atoms was recorded after a hold time of 150 ms in the trap at a constant magnetic field. Interspecies losses show up as correlated features in the loss spectra of both species.

A broad loss feature appears for both species about 0.5 G below the resonance center, where we estimate a scattering length of roughly $+3000\,a_0$. This features resembles observations made in spin mixtures of $^6$Li [11–13]

and $^{40}$K [14] and indicates the formation of weakly bound dimers, which after secondary collisions decay to deeply bound molecular states. The fact that such losses appear not at the center of the resonance, but on the side with large positive scattering length, is intrinsic to two-component fermion systems near broad Feshbach resonances with strong Pauli suppression of inelastic few-body processes.

The loss spectrum also reveals several narrow interspecies features. Some of them appear as resolved resonances, but other structures rather resemble a fluctuating background. In between features of increased losses, good regions can be identified where the lifetime exceeds 100 ms. Besides interspecies losses, we have observed intraspecies losses for Dy. This can be seen from the background atom number ($N_{\mathrm{Dy}} \approx 9500$) in Fig. 5, which is a factor of 2.5 below the initial atom number. These Dy losses generally show a fluctuating background behavior, as observed in [15].

From the timescale of losses (on the order of 100 ms), we conclude that recombination processes are no problem for experiments on short time scales (typically below 10 ms), such as the hydrodynamic expansion studied in the main text. For experiments on longer timescales, however, it may be important to choose good spots, where both intraspecies and Dy interspecies losses are minimized. The data of Fig. 5 in the main text were recorded on such a spot at 217.5 G.

### B. Model for fitting decay curves

For extracting three-body rate coefficients from atom number decay curves, one has to take into account the heating of the sample [16]. Our simple model to avoid this complication is based on the initial behavior near $t = 0$, which can be characterized by the initial number $N_0 = N(t = 0)$ and the initial decay rate $1/\tau = -\dot{N}(0)/N(0)$. To extract optimum values for these parameters from a fit to the observed decay, we follow a heuristic approach based on the differential equation

$$\frac{\dot{N}}{N_0} = -\frac{1}{\tau}\left(\frac{N}{N_0}\right)^{\alpha}, \tag{8}$$

where the phenomenological exponent $\alpha$ is a fit parameter, which absorbs possible heating and other effects. We find that the solution

$$N(t) = \frac{N_0}{\sqrt[\alpha-1]{1 + (\alpha - 1)\,t/\tau}} \tag{9}$$

fits our loss curves for all single- and mixed-species cases very well and is thus applied to all cases discussed in the present work. The calculation of rate coefficients is then based on the values for the fit parameters $N_0$ and $\tau$.

### C. Decay of K in the mixture

Here we analyze losses of K observed in the Dy-K mixture in terms of three-body processes and extract upper limits for the corresponding rate coefficients. Three-body decay of K alone is known to be very weak and can be neglected here.

We first assume that losses are caused by processes involving one K and two Dy atoms. This leads to the loss equation

$$\dot{N}_{\mathrm{K}} = -K' \int d^3r\, n_{\mathrm{K}} n_{\mathrm{Dy}}^2\,. \tag{10}$$

We approximate the number density distributions $n_i$ ($i =$ K, Dy) in the harmonic trap (mean frequencies $\bar{\omega}_i$) by thermal Gaussian distributions with spatial widths $\sigma_i = \bar{\omega}_i^{-1}\sqrt{k_B T/m_i}$. After integration we obtain

$$\frac{\dot{N}_{\mathrm{K}}}{N_{\mathrm{K}}} = -K'\, N_{\mathrm{Dy}}^2 \left(\frac{\sigma'}{2\pi\sigma_{\mathrm{K}}\sigma_{\mathrm{Dy}}^2}\right)^3, \tag{11}$$

where $\sigma' = (\sigma_{\mathrm{K}}^{-2} + 2\sigma_{\mathrm{Dy}}^{-2})^{-1/2}$.

In an analogous way, we now assume that losses are caused by processes involving two K atoms and one Dy atom (two K atoms lost per event). This leads to the loss equation

$$\dot{N}_{\mathrm{K}} = -2K'' \int d^3r\, n_{\mathrm{K}}^2 n_{\mathrm{Dy}}\,, \tag{12}$$

which after integration simplifies to

$$\frac{\dot{N}_{\mathrm{K}}}{N_{\mathrm{K}}} = -K''\, N_{\mathrm{K}} N_{\mathrm{Dy}} \left(\frac{\sigma''}{2\pi\sigma_{\mathrm{K}}^2\sigma_{\mathrm{Dy}}}\right)^3, \tag{13}$$

where $\sigma'' = (2\sigma_{\mathrm{K}}^{-2} + \sigma_{\mathrm{Dy}}^{-2})^{-1/2}$.

To obtain values (upper limits) for the event rate coefficients, we analyze the decay curves displayed in Fig. 5(a) in the main text. By using the above fit model, we extract values for the initial K decay time $\tau = -N_{\mathrm{K}}/\dot{N}_{\mathrm{K}} =$ 350(150) ms, the initial K atom number $N_{\mathrm{K}} = 3100(200)$, and the initial Dy atom number $N_{\mathrm{Dy}} = 16\,700(400)$. From Eqs. (11) and (13) and the experimental parameters ($\omega_{\mathrm{Dy}} = \omega_{\mathrm{K}}/3.6 = 2\pi \times 130\,\mathrm{Hz}$, $T = 540\,\mathrm{nK}$) we finally obtain

$$K' \approx 4 \times 10^{-25}\,\mathrm{cm}^6/\mathrm{s} \tag{14}$$
$$K'' \approx 3 \times 10^{-25}\,\mathrm{cm}^6/\mathrm{s}$$

as upper limits for the interspecies three-body event rate coefficients.

### D. Decay of Dy

Here we analyze the observed Dy decay (data shown in Fig. 5 of the main text) under the assumption that these

losses are caused by collisions of three Dy atoms. The corresponding loss equation reads

$$\dot{N}_{\rm Dy} = -3K_3 \int d^3r\, n_{\rm Dy}^3\,, \tag{15}$$

which after integration simplifies to

$$\frac{\dot{N}_{\rm Dy}}{N_{\rm Dy}} = -3K_3\, N_{\rm Dy}^2 \left(\frac{1}{2\pi\sqrt{3}\,\sigma_{\rm Dy}^2}\right)^3 . \tag{16}$$

From the fit to the Dy decay shown in Fig. 5(a) of the main text, we extract $\tau = 320(50)\,$ms and $N_{\rm Dy} = 16\,700(400)$ and obtain the value

$$K_3 = 3.4(5) \times 10^{-25}\,{\rm cm}^6/{\rm s}$$

for the event rate coefficient. Analyzing the data in Fig. 5(b) of the main text in the same way, with the fit yielding $\tau = 1000(150)\,$ms and $N_{\rm Dy} = 19\,700(400)$, we obtain the value

$$K_3 = 8.1(1.2) \times 10^{-26}\,{\rm cm}^6/{\rm s}\,.$$

The fact that he former value (with K present) is about four times larger cannot be explained by three-body loss events involving K atoms, as their contribution is too weak. However, our data show that K atoms somehow catalyze Dy losses. The underlying mechanism is currently not understood.

## III. INTERACTION-INDUCED CONTRACTION

Here we introduce a model that describes the contraction of the mixture induced by the resonant interaction in the unitarity limit under the assumption of zero temperature. The results point to a possible mechanism how the presence of K atoms can enhance three-body losses in the Dy component.

### A. Theoretical model

We calculate the number density distributions $n_{\rm Dy}(r)$ and $n_{\rm K}(r)$ of the trapped interacting species in the Thomas-Fermi limit, in which kinetic energy terms related to density variations can be neglected and the local density approximation can be applied. This also allows us to reduce the situation to a spherical trap; the solutions can then be scaled to the real, anisotropic trap.

The functional for the total energy can be written as

$$E = \int d^3r\, (U_{\rm Dy} n_{\rm Dy} + U_{\rm K} n_{\rm K} + \epsilon_{\rm Dy} + \epsilon_{\rm K} + \epsilon_{\rm int})\,, \tag{17}$$

where $U_{\rm Dy}(r) = \frac{1}{2} m_{\rm Dy} \bar{\omega}_{\rm Dy}^2 r^2$ represents the Dy trap potential and

$$\epsilon_{\rm Dy} = \frac{3}{10}(6\pi^2)^{2/3} \frac{\hbar^2}{m_{\rm Dy}} n_{\rm Dy}^{5/3} \tag{18}$$

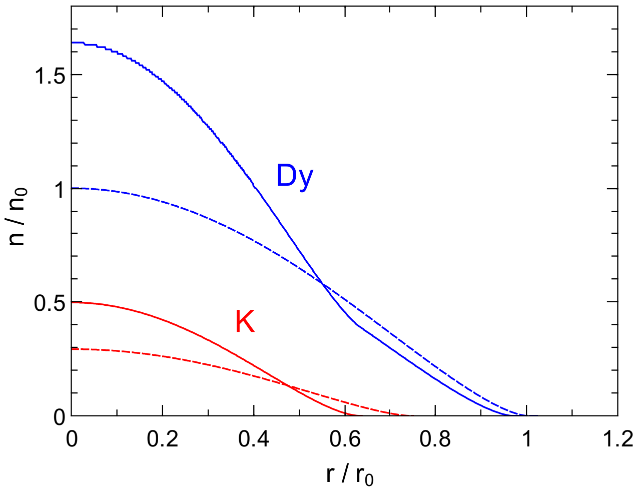


FIG. 6. Radial density distributions for the Dy and K components, with (solid lines) and without (dashed lines) interaction for a number ratio $N_{\rm K}/N_{\rm Dy} = 0.12$. All profiles are normalized to the quantities $r_0$ and $n_0$, which represent the Thomas-Fermi radius and the central density of the non-interacting Dy component, respectively.

denotes the kinetic energy density of Dy without interaction. For the K component, $U_{\rm K}$ and $\epsilon_{\rm K}$ are defined analogously.

For the interaction energy density we use the approximation

$$\epsilon_{\rm int} = -b \times \frac{3}{10}(6\pi^2)^{2/3} \frac{\hbar^2}{2m_{\rm r}} \frac{n_{\rm Dy} n_{\rm K}}{(n_{\rm Dy}^2 + n_{\rm K}^2)^{1/6}}\,. \tag{19}$$

This expression was introduced in [17] to fit the equation of state of a non-superfluid mass-balanced system [18]. Remarkably, we noticed that the same expression also provides a very good fit to the equation of state for the imbalanced mixture with mass ratio 40/6, which was published in [19]. The only difference seems to be a slight difference in the optimum value of the prefactor $b$. While $b = 1.01$ provides an optimum fit for the mass-balanced case [17], we found the slightly higher value $b = 1.04$ for the mass-imbalanced (40/6) case. In the representation of Eq. (19), the interaction term seems to be nearly independent of the mass ratio. Therefore, we are confident that it can be readily applied also to our mass ratio of 161/40.

The number density distributions $n_{\rm Dy}(r)$ and $n_{\rm K}(r)$ are found by minimizing the energy functional. This is done by varying the densities with the gradient descent method under the constraint that the atom numbers $N_{\rm Dy}$ and $N_{\rm K}$ are fixed. We represent the densities on a spatial grid, of which the step size is below $10^{-3}$ of the typical Thomas-Fermi radius of the clouds. The number of iterations in the minimization algorithm guarantees a relative precision of $10^{-4}$ for number densities and derived quantities.

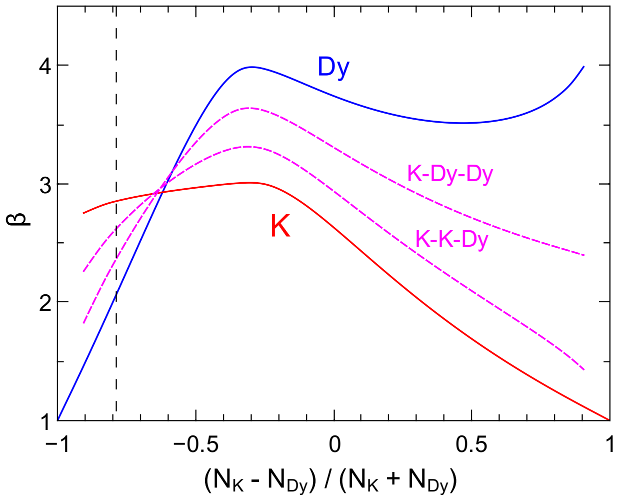


FIG. 7. Enhancement factors for three-body recombination as a function of the global polarization. The solid curves refer to intraspecies three-body collisions of Dy and K, while the dashed curves refer to interspecies processes involving both atoms. The vertical dashed line corresponds to the situation shown in Fig. 6.

### B. Density increase and loss enhancement

Figure 6 shows the effect of interaction for $N_{\mathrm{K}}/N_{\mathrm{Dy}} = 0.12$, which has been chosen to demonstrate that even a small fraction of K atoms can have a considerable effect. The interaction-induced contraction is clearly seen in profiles. The central Dy (K) density is increased by a factor of 1.64 (1.70). To quantify the total enhancement of three-body decay of Dy and K within the whole trap, we relate the total three-body decay rate to the case without interspecies interaction (Thomas-Fermi profile $n_{\mathrm{TF}}$), and define the corresponding factors

$$\beta_i \equiv \frac{\int d^3r\, n_i^3(\mathbf{r})}{\int d^3r\, n_{\mathrm{TF},i}^3(\mathbf{r})}\,, \tag{20}$$

where $i$ = Dy, K. These factors can describe both the effect of attractive ($\beta > 1$) or repulsive ($\beta < 1$) interaction in the mixture, but here we focus on the case of the strong attraction on resonance. By numerical integration of the cubed density profiles of the two species we obtain $\beta_{\mathrm{Dy}} = 2.07$ and $\beta_{\mathrm{K}} = 2.85$. It is remarkable that the presence of a relatively small minority component of K can have such a large effect on the profile and thus three-body recombination rate of the majority component of Dy.

Within the assumptions of our model, the enhancement factor depends only on the atom number ratio $N_{\mathrm{K}}/N_{\mathrm{Dy}}$ and the trap frequency ratio $\bar{\omega}_{\mathrm{K}}/\bar{\omega}_{\mathrm{Dy}}$. Since, in our experiments, the latter is fixed to a value of 3.6, we can draw universal curves for $\beta_{\mathrm{Dy}}$ and $\beta_{\mathrm{K}}$ as a function of the global polarization $(N_{\mathrm{K}} - N_{\mathrm{Dy}})/(N_{\mathrm{K}} + N_{\mathrm{Dy}})$; see Fig. 7. The solid line that represents the Dy case shows a maximum value of about $\beta_{\mathrm{Dy}} = 4$ for a polarization of $-0.7$ ($N_{\mathrm{K}}/N_{\mathrm{Dy}} = 0.54$), which highlights the possible strength of the effect.


[1] A. D. Lange, K. Pilch, A. Prantner, F. Ferlaino, B. Engeser, H.-C. Nägerl, R. Grimm, and C. Chin, Phys. Rev. A **79**, 013622 (2009).
[2] K. Jachymski and P. S. Julienne, Phys. Rev. A **88**, 052701 (2013).
[3] K. M. O'Hara, S. L. Hemmer, S. R. Granade, M. E. Gehm, J. E. Thomas, V. Venturi, E. Tiesinga, and C. J. Williams, Phys. Rev. A **66**, 041401 (2002).
[4] S. Jochim, M. Bartenstein, G. Hendl, J. Hecker Denschlag, R. Grimm, A. Mosk, and W. Weidemüller, Phys. Rev. Lett **89**, 273202 (2002).
[5] C. Chin, R. Grimm, P. S. Julienne, and E. Tiesinga, Rev. Mod. Phys. **82**, 1225 (2010).
[6] A. Mosk, S. Kraft, M. Mudrich, K. Singer, W. Wohlleben, R. Grimm, and M. Weidemüller, Appl. Phys. B **73**, 791 (2001).
[7] C. Ravensbergen, V. Corre, E. Soave, M. Kreyer, E. Kirilov, and R. Grimm, Phys. Rev. A **98**, 063624 (2018).
[8] J. R. Taylor, *An Introduction to Error Analysis* (University Science Books, 1997).
[9] D. S. Petrov, Phys. Rev. Lett. **93**, 143201 (2004).
[10] M. Jag, M. Cetina, R. S. Lous, R. Grimm, J. Levinsen, and D. S. Petrov, Phys. Rev. A **94**, 062706 (2016).
[11] K. Dieckmann, C. A. Stan, S. Gupta, Z. Hadzibabic, C. H. Schunck, and W. Ketterle, Phys. Rev. Lett. **89**, 203201 (2002).
[12] T. Bourdel, J. Cubizolles, L. Khaykovich, K. M. F. Magalhães, S. J. J. M. F. Kokkelmans, G. V. Shlyapnikov, and C. Salomon, Phys. Rev. Lett. **91**, 020402 (2003).
[13] S. Jochim, *Bose-Einstein Condensation of Molecules*, Ph.D. thesis, Innsbruck University (2004).
[14] C. A. Regal, M. Greiner, and D. S. Jin, Phys. Rev. Lett. **92**, 083201 (2004).
[15] N. Q. Burdick, Y. Tang, and B. L. Lev, Phys. Rev. X **6**, 031022 (2016).
[16] T. Weber, J. Herbig, M. Mark, H.-C. Nägerl, and R. Grimm, Phys. Rev. Lett. **91**, 123201 (2003).
[17] K. Gubbels and H. Stoof, Phys. Rep. **525**, 255 (2013).
[18] C. Lobo, A. Recati, S. Giorgini, and S. Stringari, Phys. Rev. Lett. **97**, 200403 (2006).
[19] A. Gezerlis, S. Gandolfi, K. E. Schmidt, and J. Carlson, Phys. Rev. Lett. **103**, 060403 (2009).
